# Supplementary material for: Few-Shot Class-Incremental Learning via Entropy-Regularized Data-Free Replay
Source: arXiv:2207.11213 source file (2022-07-22)
Supplement: Supplementary file 1 [file appendix.tex]

\clearpage
\appendix
\section{Overall Algorithm}
In this section, we demonstrate the overall algorithm for a better understanding of our proposed method. At the beginning of each session, we first train a generator given the old model from the previous session. After the training of the generator, we then conduct incremental learning following Section 4.2, where we form a new dataset by combining the novel data with the relabeled replayed data and only use the cross-entropy loss to learn novel classes and avoid forgetting of old classes. 

\begin{algorithm}[h]
\footnotesize
\caption{Entropy-regularized Data-free FSCIL}\label{alg:main}
\begin{algorithmic}[1]
\Require $\mathcal{T}_i(\cdot;\theta_i)$, $\mathcal{A}_i(\cdot;\theta_{A_i})$, $\mathcal{G}_i(\cdot;\theta_{G_i})$: models
\Require $\alpha, \beta, \lambda_1, \lambda_2$ : learning rates
\Require $\{\mathcal{D}_{train}^0, \mathcal{D}_{train}^1, ..., \mathcal{D}_{train}^N \}$ : datasets
\State Base training of  $\mathcal{T}_0(\cdot;\theta_{0})$ on $\mathcal{D}_{train}^0$ \Comment{Session 0.}
\For{$i = 1,...,N$} \Comment{Loop through all the sessions.}
\State \textbf{1. Training Generator using entropy regularization.}
\While{\textit{not converge}}
\State $z \sim \mathcal{N}(0, I)$ \Comment{Sampling noise vector.}
\For{k iterations}
% \State {\tiny $\mathcal{L}_G^* = -||\mathcal{T}_{i-1}(\mathcal{G}_i(z)) - \mathcal{S}_i(\mathcal{G}_i(z))||_1 - H(\mathcal{T}_{i-1}(\mathcal{G}_i(z)))$} 
% \Comment{Calculate loss with entropy constraint.}
\State $\theta_{G_i} \leftarrow \theta_{G_i} - \alpha  \frac{\partial \mathcal{L}_{G}^*}{\partial \theta_{G_i}}$ \Comment{Update generator.}
\EndFor
% \State $\mathcal{L}_S = ||\mathcal{T}_i(\mathcal{G}_i(z)) - \mathcal{S}_i(\mathcal{G}_i(z))||_1$
\State $\theta_{A_i} \leftarrow \theta_{A_i} - \beta  \frac{\partial \mathcal{L}_{A}}{\partial \theta_{A_i}}$ \Comment{Update auxiliary model.}
\EndWhile
\State \textbf{2. Learning incrementally with uncertain data.}
\State initialize $\mathcal{T}_i(\cdot;\theta_i)$ by $\mathcal{T}_{i-1}(\cdot;\theta_{i-1})$
\While{\textit{not converge}}
\State $x^* \leftarrow \mathcal{G}_i(z;\theta_{G_i})$ \Comment{Generate data for replaying.}
\State $y^* \leftarrow argmax (\mathcal{T}_{i-1}(x^*))$ \Comment{labeling $x^*$ by old model's activation.}
\State  $\mathcal{D}_{train^*}^i \leftarrow \mathcal{D}_{train}^i \cup \{x^*, y^*\}$ \Comment{Update dataset.}
\State Sample $\{x, y\}$ from $\mathcal{D}_{train^*}^i$
\State $\{\theta^b_{i-1}, \theta^{l}_{i-1}\} = \{\theta^b_{i-1}, \theta^{l}_{i-1}\} - \lambda_1  \frac{\partial \mathcal{L}_{CE}}{\partial \{\theta^b_{i-1}, \theta^{l}_{i-1}\}}$ \Comment{Fine-tuning old parameters.}
\State $\theta^{l^*}_i = \theta^{l^*}_i - \lambda_2  \frac{\partial \mathcal{L}_{CE}}{\partial \theta^{l^*}_i}$ \Comment{Update new parameters.}

\EndWhile
\State   
$\theta_{i} = \{\theta^b_i, \theta^{l}_i\}$, where $\theta^{l}_i = \{\theta^{l}_{i-1}\, \theta^{l^*}_i\}$
\EndFor

\State \Return $\mathcal{T}_N(\cdot;\theta_N)$
\end{algorithmic}
\end{algorithm}
